# Supplementary material for: SafeCoEvo: Co-Evolving Safety Harnesses and Guards for LLM Agents at Test-Time
Source: arXiv:2609.36580 source file (2026-10-02)
Supplement: Supplementary file 1 [file appendix_prompts.tex]

% Insert after all existing appendix material, including the trajectory example.
% The main paper has already called \appendix. Do NOT call it again here.
\clearpage
\section{Prompts for Target Agent and S-Harness Evolution}
\label{app:safecoevo-prompts}

This appendix documents the Target Agent system addendum and the Evolution
Agent prompt templates for S-Harness. The Target Agent completes the original
user task with guidance from the runtime Safety Harness. After an episode is
completed, the Evolution Agent uses its execution evidence, official feedback,
and current harness artifacts to propose reusable content updates for future
episodes. This separation implements the short-timescale adaptation described
in Section~3.2; it does not update the task-performing model's parameters or
perform the GuardVPO parameter update.

The listings reproduce the supplied implementation snapshot, including its
placeholders, examples, and comment markers. The Target Agent listing is a
system addendum rather than the complete task-specific system message. The
Evolution Agent system listing is the exported default rendering with
\texttt{include\_permission\_policy=False} and the patch template inserted.
Task-specific user messages, retrieved content, and episode evidence are
runtime inputs and are not expanded here.

\subsection{Target Agent: Runtime System Addendum}
\label{app:safecoevo-target-prompt}

The addendum defines how the Target Agent interprets harness guidance while
pursuing the original user task. It specifies tool-use discipline, task-progress
tracking, authorization and feasibility checks, and the interpretation of
Guard feedback. The placeholder
\texttt{\{\{HARNESS\_ARTIFACTS\}\}} is reserved for runtime harness content.
The source is \path{DEFAULT_HARNESS_SYSTEM_ADDENDUM} in
\path{target_prompts.py}.

\SafeCoEvoPromptFile{Target Agent: system addendum}{prompts/target_system_addendum.txt}

\subsection{Evolution Agent: System Prompt}
\label{app:safecoevo-evolution-system}

The Evolution Agent operates between completed and future episodes. Its system
prompt limits updates to the contents of the existing Prompt, Memory, Skill,
Permission, and Guard Policy artifact categories. It specifies evidence use,
component selection, reusable-update criteria, and the patch output contract.
Official feedback provides the outcome supervision for the completed episode,
while Guard observations are treated as fallible supporting evidence. Candidate
validation checks patch structure and does not replay completed tasks. The
source is \path{evolution_agent_system_prompt()} in
\path{evolution_graph.py}.

\SafeCoEvoPromptFile{Evolution Agent: system prompt}{prompts/evolution_system.txt}

\subsection{Evolution Agent: User-Message Template}
\label{app:safecoevo-evolution-user}

The user-message template supplies the completed-episode evidence and the state
against which an update is proposed. Runtime fields provide the task identifier,
evidence, current artifacts, artifact update contract, prior patch history,
workspace description, and patch schema. These fields are retained as
placeholders so that the template remains distinct from any particular episode.
The template is stored in
\path{prompt_templates/evolution_agent/user_prompt.md}.
It is populated by \path{evolution_agent_user_prompt()}.

\SafeCoEvoPromptFile{Evolution Agent: user-message template}{prompts/evolution_user_template.txt}
